# Supplementary material for: Topologically distinct atomic insulators
Source: arXiv:2211.09804 ancillary file (2023-07-24)
Supplement: Supplementary file 1 [file suppl.pdf]

# Supplemental Material: Topologically distinct atomic insulators

Sanjib Kumar Das,[1] Sourav Manna,[2,3] and Bitan Roy[1]
[1]*Department of Physics, Lehigh University, Bethlehem, Pennsylvania, 18015, USA*
[2]*Department of Condensed Matter Physics, Weizmann Institute of Science, Rehovot 7610001, Israel*
[3]*Raymond and Beverly Sackler School of Physics and Astronomy, Tel-Aviv University, Tel Aviv 6997801, Israel*
(Dated: June 29, 2023)

In this Supplemental Material, we present (a) additional details for transport simulations [Sec. S1 and Fig. S1], (b) energy dependence of the integrand function for various temperatures as mentioned in the Eq. (3) of the main manuscript [Sec. S2 and Fig. S2], and (c) computation of the weak topological invariant, namely the Zak phase, for the 'weak TSC' phase appearing in the phase diagram from Fig. 2(a) of the main manuscript [Sec. S3], realization of topological superconductivity at smaller pairing amplitude at finite chemical doping [Sec. S4 and Fig. S3], an emergent 'inversion' symmetry of the normal state Hamiltonian [Sec. S5], topological superconductivity for infinitesimal pairing amplitude near the Fermi surface [Sec. S6], and disorder-averaged robust longitudinal thermal conductance ($G_{th}$) and thermal Hall conductivity ($\kappa_{xy}$) [Sec. S7 and Fig. S4].

## S1. ELECTRICAL AND THERMAL HALL TRANSPORT SETUP

In this section, we present the transport geometry which we briefly mentioned in the main manuscript. As a side remark, as we are dealing with two-dimensional system, conductance and conductivity are synonymous. For calculating both the electrical and thermal Hall conductances, we consider a rectangular scattering geometry with six symmetric leads attached to the scattering region in Kwant [1] as shown in Fig. S1. The semi-infinite periodic leads are connected to the external reservoirs, and provided with propagating electronic channels which enter into the scattering region. Since the leads have translation invariance, the propagating channels in the lead are composed of plane waves. Therefore, these modes can get reflected back into the same lead that it came from, or they can get transmitted into other leads. This process is fully captured by the unitary scattering matrix

$$S = \begin{pmatrix} r & t' \\ t & r' \end{pmatrix}, \tag{S1}$$

where, $r$ and $r'$ ($t$ and $t'$) are the reflection (transmission) blocks of the scattering matrix. Since we have six leads

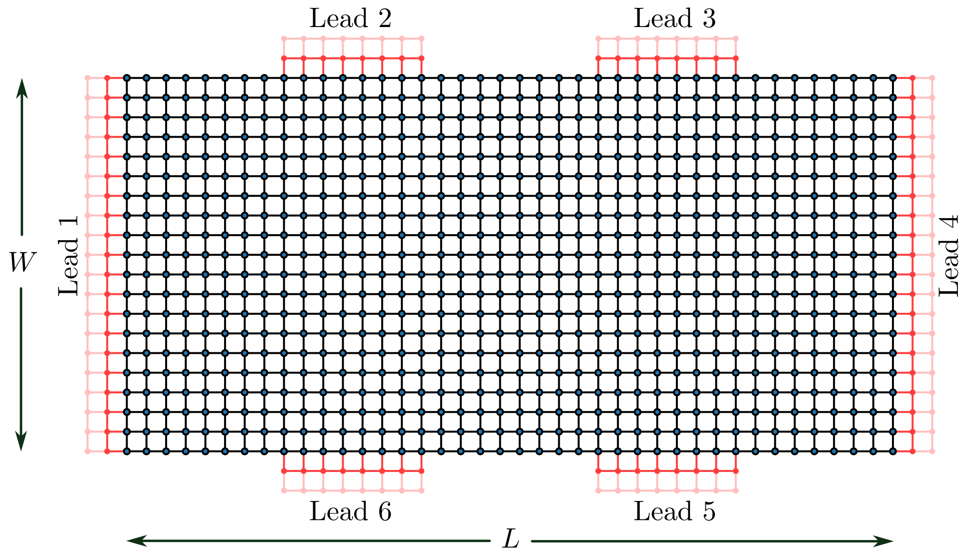


Figure S1. Schematic of the six terminal rectangular transport geometry. Leads are indicated by red colored sites, and the scattering region consists of blue sites. Here $L$ and $W$ correspond to the length and width of the rectangular system, respectively.

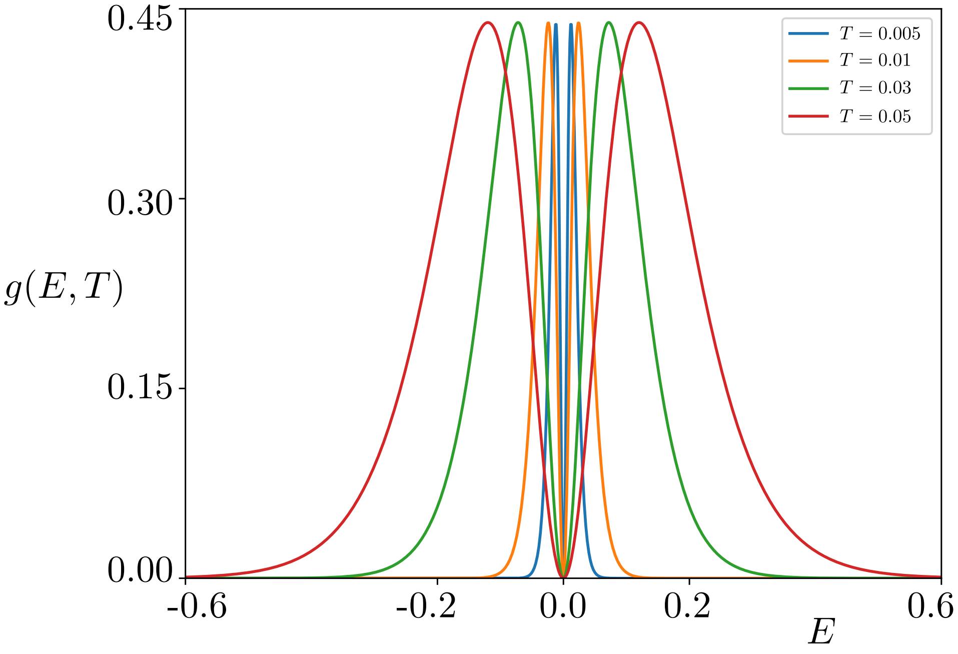


Figure S2. $g(E,T)$ [Eq. (S3)] as a function of energy is plotted for various choices of the temperature $T$. Values of $T$ are taken in the units of $t$ which define the energy scale of the problem.

present in the system, the scattering matrix in Eq. (S1) has $6 \times 6$ block structure, encapsulating all possible matrix elements between different leads. In our calculation, leads have propagating electronic modes, with the same degrees of freedom as that of the system per site (two in case of Eq. (1) and four in case of Eq. (4) of the main manuscript). This construction allows the modes to be reflected or transmitted at the boundaries.

Let us describe the simple situation how one can calculate six terminal electrical Hall response. As there is a current ($\boldsymbol{j}$) flowing across the system in presence of an applied electric field ($\boldsymbol{E}$), the current-electric field relation reads $j_a = \sum_b \sigma_{ab} E_b$, where $\sigma_{ab}$ is called the conductivity tensor. Since in our setup (Fig. S1), current is only flowing along the $x$-direction between Lead 1 and Lead 4, one can probe the off-diagonal components of the conductivity tensor from the voltage drop between Lead 2, Lead 3, Lead 5 and Lead 6. Finally, the Hall conductivity can be written as

$$\sigma_{H} = \frac{j_x E_y}{E_x^2 + E_y^2}, \tag{S2}$$

where $E_x = V_2 - V_3$, $E_y = (V_2 + V_3 - V_5 - V_6)/2$, and $V_i$ is the voltages developed in the $i$th lead.

## S2. NATURE OF THE INTEGRAND IN THE COMPUTATION OF $\kappa_{xy}$

In this section, we will investigate the nature of the integrand presented in Eq. (3) of the main text. Since the integrand is temperature dependent, it is crucial to inspect the product of $E/T$ and the derivative of the Fermi-Dirac function $\partial f(E,T)/\partial E$ which enters into the integral. The function of our interest is

$$\begin{aligned} g(E,T) &= \frac{E^2}{T}\left(-\frac{\partial f(E,T)}{\partial E}\right) \\ &= \frac{E^2}{T^2}\frac{e^{E/T}}{(1+e^{E/T})^2}, \end{aligned} \tag{S3}$$

where $f(E,T) = 1/(1+e^{E/T})$ is the Fermi-Dirac function. We have set the Boltzmann constant $k_B = 1$ throughout. From Fig. S2, we note that the function $g(E,T)$ gets broader with increasing temperature. It is also important to

notice that the energy integrand turns out to be almost zero beyond a certain range of energy after the function has decayed completely, which in turn allows the integral [Eq. (3) of the main manuscript] to be evaluated only in a certain energy window. The presented thermal Hall results in the main manuscript are carried out with the function $g(E, 0.01)$.

## S3. TOPOLOGICAL INVARIANT OF 'weak TSC' PHASE

Before we delve into the computation of the topological invariant of the two-dimensional (2D) 'weak TSC' phase appearing in the phase diagram from Fig. 2(a) of the main manuscript, we show the calculation of the Zak phase of the one-dimensional (1D) Su–Schrieffer–Heeger model, captured by the Bloch Hamiltonian

$$\mathcal{H}_{\rm SSH}(k_x) = \tau_1 d_1(k_x) + \tau_2 d_2(k_x), \tag{S4}$$

with $d_1(k_x) = t\sin(k_x a)$ and $d_2(k_x) = m + t_1\cos(k_x a)$. We set the lattice spacing $a = 1$. One can write $d_1(k_x) \pm d_2(k_x) = |\boldsymbol{d}(k_x)|\ \exp[\pm i\phi_{k_x}]$, where $\phi_{k_x} = \tan^{-1}(d_2(k_x)/d_1(k_x))$ and $|\boldsymbol{d}(k_x)| = [d_1^2(k_x) + d_2^2(k_x)]^{1/2}$. The topological invariant, namely the Zak phase, of this model is defined as

$$\Phi_{\rm Zak} = \int_{-\pi}^{\pi} \frac{dk_x}{2\pi}\, \frac{\partial \phi_{k_x}}{\partial k_x}. \tag{S5}$$

Within the parameter regime $-1 \leq m/t_1 \leq 1$, $\Phi_{\rm Zak} = 1$ (topological), while $\Phi_{\rm Zak} = 0$ (trivial) for $|m/t_1| > 1$. The nontrivial Zak phase manifests through the endpoint zero energy modes. Next we use this definition to find the weak topological invariant of a 2D TSC.

In the main manuscript, we have already shown that the Bogoliubov de Gennes (BdG) Hamiltonian for the only local pairing can be cast in a block diagonal form (after a suitable unitary rotation by $U$), $\mathcal{H}^{+}_{\rm BdG}(\boldsymbol{k}) \oplus \mathcal{H}^{-}_{\rm BdG}(\boldsymbol{k})$, where

$$\mathcal{H}^{\pm}_{\rm BdG}(\boldsymbol{k}) = \tau_1 d_1(\boldsymbol{k}) + \tau_2 d_2(\boldsymbol{k}) + \tau_3 d_3^{\pm}(\boldsymbol{k}), \tag{S6}$$

with $d_1(\boldsymbol{k}) = t\sin(k_x a)$, $d_2(\boldsymbol{k}) = t\sin(k_y a)$ and $d_3^{\pm}(\boldsymbol{k}) = m_0 \pm \Delta - t_0[\cos(k_x a) + \cos(k_y a)]$. Weak invariant of a 2D TSC is computed over a 1D Brillouin zone in the $x$ direction, for example, at high symmetry points $k_y = 0$ and $\pi$ in the orthogonal direction. At these two high symmetry points, we define effective 1D BdG Hamiltonian as

$$\mathcal{H}^{\pm}_{\rm BdG}(k_x, 0) = \tau_1 d_1(k_x) + \tau_3 d_3^{\pm}(k_x, 0) \quad \text{and} \quad \mathcal{H}^{\pm}_{\rm BdG}(k_x, \pi) = \tau_1 d_1(k_x) + \tau_3 d_3^{\pm}(k_x, \pi), \tag{S7}$$

respectively. After a unitary rotation by $U_1 = \exp[-i\pi\tau_1/4]$, we can cast $\mathcal{H}^{\pm}_{\rm BdG}(k_x, 0)$ and $\mathcal{H}^{\pm}_{\rm BdG}(k_x, \pi)$ in the form of Eq. (S4), namely

$$U_1^\dagger \mathcal{H}^{\pm}_{\rm BdG}(k_x, 0) U_1 = \tau_1 d_1(k_x) + \tau_2 d_3^{\pm}(k_x, 0), \quad \text{and} \quad U_1^\dagger \mathcal{H}^{\pm}_{\rm BdG}(k_x, \pi) U_1 = \tau_1 d_1(k_x) + \tau_2 d_3^{\pm}(k_x, \pi), \tag{S8}$$

respectively. We now define the following Zak phases for various blocks ($\pm$) and different values of $k_y$ (0 and $\pi$)

$$\Phi^{\pm}_{\rm Zak}(0) = \int \frac{dk_x}{2\pi}\, \frac{\partial \phi^{\pm}_{k_x}(0)}{\partial k_x} \quad \text{and} \quad \Phi^{\pm}_{\rm Zak}(\pi) = \int \frac{dk_x}{2\pi}\, \frac{\partial \phi^{\pm}_{k_x}(\pi)}{\partial k_x}, \tag{S9}$$

where $\phi^{\pm}_{k_x}(0) = \tan^{-1}(d_3^{\pm}(k_x, 0)/d_1(k_x))$ and $\phi^{\pm}_{k_x}(\pi) = \tan^{-1}(d_3^{\pm}(k_x, \pi)/d_1(k_x))$. In the 'weak TSC' phase we find $\Phi^{+}_{\rm Zak}(0) = \Phi^{-}_{\rm Zak}(\pi) = 1$. The computation of the weak invariant can also be performed over the 1D Brillouin zone in the $k_y$ direction for $k_x = 0$ and $\pi$. It leads to identical conclusions. As a consequence of possessing such weak topological invariants, the 'weak TSC' phase supports topologically protected edge modes crossing the zero energy at $k_j = 0$ and $\pi$, where $j = x$ or $y$, as shown in Fig. 3(b) of the main manuscript, and a single pair of dislocation modes following the $\mathbf{K} \cdot \mathbf{b}$ rule, as shown in Fig. 4(c) of the main manuscript.

## S4. TOPOLOGICAL SUPERCONDUCTIVITY AT FINITE CHEMICAL DOPING

In this section we argue that when the system is doped, the topological superconductivity (TSC) can be realized for weaker pairing amplitudes in comparison to those at zero chemical doping. The results are summarized in Fig. S3.

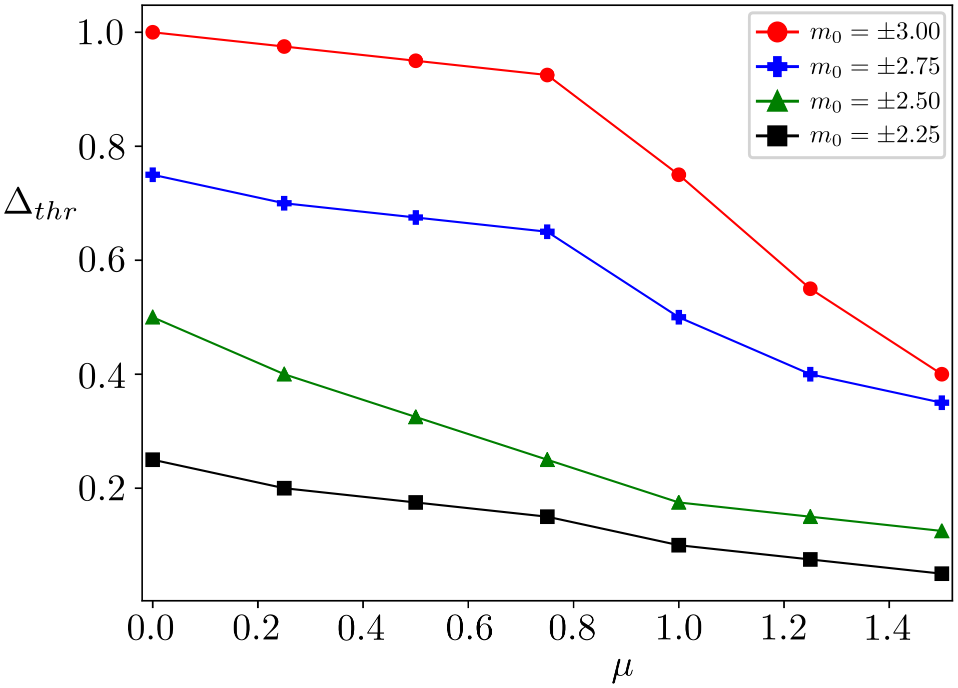


Figure S3. The threshold pairing amplitude ($\Delta_{thr}$) only above which TSC can be realized as function of the chemical doping for various choice of $m_0$, such that the system is always in the NI phase in the absence of any pairing. The TSC is identified from integer Bott index (see Sec. S4)) computed in a $20 \times 20$ square lattice.

At finite doping, the effective single-particle BdG Hamiltonian can not be cast in a block diagonal form. Therefore, to identify TSC, we compute the Bott index [2]. We place all the sites of the square lattice within a unit square, and denote their coordinates by $x_i \in [0,1]$ and $y_i \in [0,1]$. Subsequently, we define two diagonal matrices $X_{i,j} = x_i \delta_{i,j}$ and $Y_{i,j} = y_i \delta_{i,j}$, and two diagonal unitary matrices $U_x = \exp(2\pi i X)$ and $U_y = \exp(2\pi i Y)$. Finally, in terms of the projector ($\mathcal{P}$) onto the filled eigenstates of the effective single-particle BdG Hamiltonian up to the Fermi energy ($\mu$), defined as $\mathcal{P} = \sum_{E<\mu} |E\rangle\langle E|$, we compute

$$B = \frac{1}{2\pi} \text{Im} \left[ \text{Tr} \left[ \ln \left[ V_x V_y V_x^\dagger V_y^\dagger \right] \right] \right], \tag{S10}$$

where $V_j = I - \mathcal{P} + \mathcal{P} U_j \mathcal{P}$ for $j = x$ and $y$. For TSC $B = \pm 1$, while for trivial superconductors $B = 0$. In terms of the Bott index we identify the threshold pairing amplitude ($\Delta_{thr}$) above which TSC sets in as a function of the chemical doping ($\mu$) for various values of $m_0$ such that the normal state is always a trivial insulator. We find that irrespective of whether the band gap minima of the NI is around the $\Gamma$ or the M point, with increasing doping $\Delta_{thr}$ always decreases. Therefore, our proposal to identify the parent NIs from the topological responses of the proximal paired state remain operative even away from the TI-NI critical point for weak pairing amplitude as long as the system is sufficiently doped.

## S5. EMERGENT INVERSION SYMMETRY

Often topological materials and models result from the hybridization between two orbitals with opposite parities [3], which is also the case for the Qi-Wu-Zhang model, we consider in this work. The Hamiltonian takes the schematic form $H = \sum_{\boldsymbol{k}} \Psi^\dagger_{\boldsymbol{k}} \mathcal{H}(\boldsymbol{k}) \Psi_{\boldsymbol{k}}$. For the sake of simplicity, we assume two involved orbitals to be $s$ and $p$ type, with the wavefunctions $\Psi_s(\boldsymbol{k})$ and $\Psi_p(\boldsymbol{k})$, respectively, satisfying the parity symmetries: $\Psi_s(-\boldsymbol{k}) = \Psi_s(\boldsymbol{k})$ and $\Psi_p(-\boldsymbol{k}) = -\Psi_p(\boldsymbol{k})$. The Hamiltonian operator is $\mathcal{H}(\boldsymbol{k}) = \boldsymbol{\tau} \cdot \boldsymbol{d}(\boldsymbol{k})$. We seek to find the symmetry of the components of the $\boldsymbol{d}$ vector, given by $\boldsymbol{d}(\boldsymbol{k}) = (d_1(\boldsymbol{k}), d_2(\boldsymbol{k}), d_3(\boldsymbol{k}))$, such that their expectation values are nontrivial, when computed within

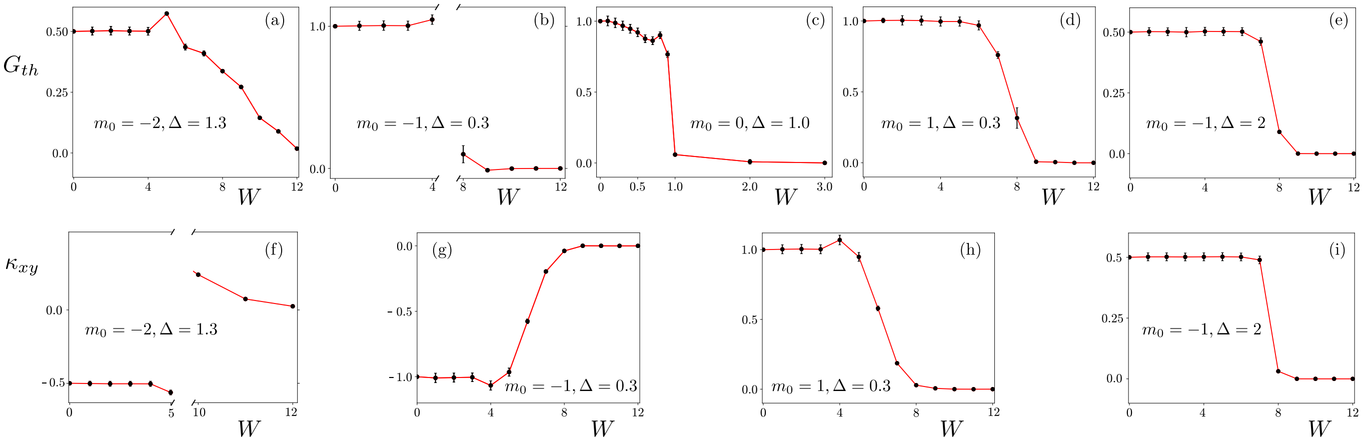


Figure S4. Robustness of the longitudinal thermal conductance $G_{th}$ (upper panel) and the transverse thermal Hall conductivity $\kappa_{xy}$ (lower panel) in the presence of on-site disorder (random charge impurities). The system size for the disorder-averaged calculations of $G_{th}$ and $\kappa_{xy}$ is $L = 2W = 80$ and set the temperature $T = 0.01$. We average over 20 random and independent disorder realizations for all the cases and sufficiently small error bars ensure convergence of all the results. Here $W$ corresponds to the disorder strength. The parameter values for the lattice model are quoted in the inset of each figure. See also Fig. 2(a) of the main manuscript for the phase diagram, characterizing all the paired states, and Fig. 2(b) of the main manuscript for the values of $G_{th}$ and $\kappa_{xy}$ in the clean system ($W = 0$). See Sec. S7 for details.

the subspace of two orbitals with opposite parities. Explicitly, we find

$$\begin{aligned}
\langle d_1(\boldsymbol{k})\tau_1\rangle &= \sum_{\boldsymbol{k}} \Psi_s^\star(\boldsymbol{k}) d_1(\boldsymbol{k}) \Psi_p(\boldsymbol{k}) + H.c. \neq 0 \quad \text{if and only if} \quad d_1(-\boldsymbol{k}) = -d_1(\boldsymbol{k}), \\
\langle d_2(\boldsymbol{k})\tau_2\rangle &= -i\sum_{\boldsymbol{k}} \Psi_s^\star(\boldsymbol{k}) d_2(\boldsymbol{k}) \Psi_p(\boldsymbol{k}) + H.c. \neq 0 \quad \text{if and only if} \quad d_2(-\boldsymbol{k}) = -d_2(\boldsymbol{k}), \\
\text{and} \quad \langle d_3(\boldsymbol{k})\tau_3\rangle &= \sum_{\boldsymbol{k}} \Psi_s^\star(\boldsymbol{k}) d_3(\boldsymbol{k}) \Psi_s(\boldsymbol{k}) - (s \leftrightarrow p) \neq 0 \quad \text{if and only if} \quad d_3(-\boldsymbol{k}) = d_3(\boldsymbol{k}).
\end{aligned} \tag{S11}$$

Therefore, $H \neq 0$ when $d_1(\boldsymbol{k})$ and $d_2(\boldsymbol{k})$ are odd under the spatial inversion, while $d_3(\boldsymbol{k})$ is even under it. This requirement is mandated by the symmetry of the involved orbitals. One choice of the $\boldsymbol{d}$-vector that satisfies these symmetry criteria is shown in Eq. (1) of the main manuscript. With these symmetry requirements of the components of the $\boldsymbol{d}$-vector, the operator $\mathcal{H}(\boldsymbol{k})$ enjoys an 'emergent' inversion symmetry, generated by $\tau_z$, under which $\boldsymbol{k} \to -\boldsymbol{k}$. It should be noted that this symmetry was not imposed a priory. The parities of the involved orbitals give rise to such symmetry, and hence it is not a microscopic symmetry, rather an emergent one. As a matter of fact, all the model Hamiltonian from any Altland-Zirnbauer symmetry class in any dimension enjoy such emergent 'inversion' symmetry, resulting solely from the parities of the involved orbitals [3].

## S6. TOPOLOGICAL PAIRING IN THE FERMI SURFACE

In Sec. S4, we have shown that the threshold pairing amplitude for topological superconductivity ($\Delta_{thr}$) decreases monotonically once the system is doped (i.e., when $\mu$ is finite). However, due to inter-band scattering $\Delta_{thr}$ remains finite [Fig. S3]. Here we show that within the BCS pairing mechanism, in which the attractive pairing interaction exists only in the close vicinity of the Fermi surface, realized by doping the insulating normal state, topological superconductivity can be realized for infinitesimal pairing amplitude (i.e. $\Delta_{thr} \to 0$). It can be demonstrated by considering only the intra-band piece of the pairing within the valence or conduction band, supporting the Fermi surface, while neglecting the inter-band part, which is justified within the BCS pairing picture.

To proceed, we first consider the BdG Hamiltonian $H_{\rm BdG}$ [see Eq. (4) of the main manuscript] without the pairing term ($\Delta = 0$), in the presence of a finite chemical potential ($\mu$). A unitary rotation by the diagonalizing matrix, brings this $H_{\rm BdG}$ to a diagonal form. We then isolate the pieces for the conduction band, yielding its effective Hamiltonian $H_{\rm con} = (d_3(\boldsymbol{k}) - \mu)\,\eta_3 = [-\tilde{m}_0 - t_0\{\cos(k_x a) + \cos(k_y a)\}]\,\eta_3$, where $\tilde{m}_0 = \mu - m_0$ is the effective chemical potential

measured from the bottom of the conduction band. The unitary diagonalizing matrix is obtained by columnwise arranging the eigenvectors of $H_{\rm BdG}$ with $\Delta = 0$. In arriving at the final expression, we made a simplification that $|d_3(\boldsymbol{k})| \ll |d_1(\boldsymbol{k})|, |d_2(\boldsymbol{k})|$ (large mass approximation) to keep the analysis analytically tractable.

Upon acting with the unitary diagonalizing matrix on the pairing term, when we only retain its intra-band piece within the conduction band, the effective Hamiltonian reads as

$$H^{\rm con}_{\rm pair} = \tilde{\Delta} \left[ \sin(k_x a) \eta_1 + \sin(k_y a) \eta_2 \right], \tag{S12}$$

where $\tilde{\Delta} = \Delta/|d_3(\boldsymbol{k})|$ is the reduced pairing amplitude. Together $H^{\rm BdG}_{\rm con} = H_{\rm con} + H^{\rm con}_{\rm pair}$ describes topological paired state even for an infinitesimal pairing amplitude $\Delta$, whenever a Fermi surface is formed, i.e., $\tilde{m}_0 > 0$. This conforms the weak coupling BCS pairing scenario, and the topological invariant of $H^{\rm BdG}_{\rm con}$ can readily be computed from the definition of the first Chern number [Eq. (2) of the main manuscript]. Notice that this outcome holds in the absence of any inter-band scattering caused by the pairing, which is consistent with the BCS formalism. More details on this methodology can be found in Ref. [4]. This procedure allows us to capture the TSCs with the Chern number $C = \pm 1$, which can be realized by doping normal insulators with the band gap minima near the $\Gamma$ and M points for infinitesimal pairing amplitude, which we seek to distinguish topologically by inducing topological pairing therein. However, in the absence of any inter-band scattering we cannot capture the $C = \pm 2$ paired states nor the weak-TSC phase [see Fig. 2(a) of the main manuscript].

## S7. DISORDER-AVERAGED $G_{\rm th}$ AND $\kappa_{xy}$

All the paired states appearing in Fig. 2(a) of the main manuscript are characterized by distinct topological invariant (Chern number or weak topological invariant) and concomitantly they feature distinct thermal responses, namely the longitudinal thermal conductance ($G_{th}$) and the transverse thermal Hall conductivity ($\kappa_{xy}$) in the clean system, summarized Fig. 2(b) of the main manuscript. Here we show that the (half)-quantized values of $G_{th}$ and $\kappa_{xy}$ are robust in the presence of random charge impurities, the dominant source of elastic scattering in any real material. The results are shown in Fig. S4.

The effect of random charge impurities are captured by adding the following term $V(\boldsymbol{r})\Gamma_{30}$ to the real space square lattice version of $\mathcal{H}_{\rm BdG}(\boldsymbol{k})$ [see Eq. (4) of the main manuscript]. Here $V(\boldsymbol{r})$ is distributed uniformly and randomly within the range $[-W/2, W/2]$ at each site of the square lattice. Thus, $W$ denotes the disorder strength. We compute the disorder-averaged $G_{th}$ and $\kappa_{xy}$ in a system with $L = 2W = 80$ and at a temperature $T = 0.01$. For each disorder realization, the computation of $G_{th}$ and $\kappa_{xy}$ is identical to the one we previously discussed for the clean system in details.

We are interested in the (a) weak or moderate disorder regime, where as shown in Fig. S4, $G_{th}$ and $\kappa_{xy}$ retain their (half)-quantized values (in units of $\kappa_0$) reported previously [Fig. 2(b) of the main manuscript] in the clean system ($W = 0$), and (b) strong disorder regime where both of them vanish, yielding a trivial superconductor. In these two regimes disorder averaging over 20 random realizations of $V(\boldsymbol{r})$ produces convergent results, as can be seen from the corresponding error bars in Fig. S4.

Notice that except for the weak topological superconductor (weak TSC), $G_{th}$ and $\kappa_{xy}$ remain (half)-quantized (within numerical accuracy) up to moderate disorder strengths $W \approx 4-5$, confirming their robust nature in the presence of random charge impurities. In the weak TSC phase, featuring only quantized $G_{th}$ remains robust up to $W \approx 0.1$. Notice near the disorder-driven topological to trivial superconductor quantum phase transition, $G_{th}$ and $\kappa_{xy}$ shows large fluctuations and in order to underpin the associated critical disorder strength ($W_c$) we need to perform disorder averaging over much more disorder realizations, which, however, falls outside the theme of the present work.

[1] C. W. Groth, M. Wimmer, A. R. Akhmerov, and X. Waintal, New J. Phys. **16**, 063065 (2014).
[2] S. Manna, S. K. Das, and B. Roy, arXiv:2207.02203.
[3] A. P. Schnyder, S. Ryu, A. Furusaki, and A. W. W. Ludwig, Phys. Rev. B **78**, 195125 (2008).
[4] B. Roy, Phys. Rev. B **101**, 220506 (2020).
